# Supplementary material for: Static spin exchange-correlation kernel of the uniform electron gas at finite temperature
Source: arXiv:2605.16888 source file (2026-10-14)
Supplement: Supplementary file 1 [file supplement.tex]

\documentclass[reprint,prb,aps,floatfix,superscriptaddress,nofootinbib,
  onecolumn]{revtex4-2}

\usepackage{amsmath,amssymb,graphicx,bm,booktabs}
\usepackage[colorlinks=true,linkcolor=blue,citecolor=blue,urlcolor=blue]{hyperref}

\newcommand{\rs}{r_s}
\newcommand{\kF}{k_F}
\newcommand{\TF}{T_F}
\newcommand{\Nf}{N_F}
\newcommand{\Kxc}{K^{-}_{xc}}
\newcommand{\KxcPlus}{K^{+}_{xc}}
\newcommand{\chis}{\chi_s}
\newcommand{\chinaught}{\chi_0}
\newcommand{\axc}{\alpha_{xc}}
\newcommand{\pexp}{p}
\newcommand{\fxc}{f_{xc}}
\newcommand{\thetared}{\theta}

\begin{document}

\renewcommand{\thefigure}{S\arabic{figure}}
\renewcommand{\thetable}{S\arabic{table}}
\renewcommand{\theequation}{S\arabic{equation}}

\title{\texorpdfstring{Supplemental Material:\\}{Supplemental Material: }
    Finite-Temperature Spin Exchange-Correlation Kernel of the
    Uniform Electron Gas}

\author{Pengcheng Hou}
\thanks{These two authors contributed equally to this paper.}
\affiliation{Hefei National Laboratory, University of Science and Technology of China, Hefei 230088, China}

\author{Zhiyi Li}
\thanks{These two authors contributed equally to this paper.}
\affiliation{Department of Modern Physics, University of Science and Technology of China, Hefei, Anhui 230026, China}

\author{Youjin Deng}
\email{yjdeng@ustc.edu.cn}
\affiliation{Department of Modern Physics, University of Science and Technology of China, Hefei, Anhui 230026, China}
\affiliation{Hefei National Laboratory, University of Science and Technology of China, Hefei 230088, China}

\author{Kun Chen}
\email{chenkun@itp.ac.cn}
\affiliation{CAS Key Laboratory of Theoretical Physics, Institute of Theoretical Physics, Chinese Academy of Sciences, Beijing 100190, China}

\date{\today}

\maketitle

% \tableofcontents

%% =================================================================
\section{Conventions}\label{sec:convention}
%% =================================================================

We collect here the conventions used throughout the main text and in
this Supplemental Material so that all coefficients and signs can be
unambiguously cross-checked.

\paragraph*{Atomic units.}
We work in Rydberg atomic units throughout
($\hbar=2m_e=e^2/2=1$): lengths in Bohr, energies in Rydberg,
and the bare Coulomb interaction $v(q)=8\pi/q^2$.

\paragraph*{Density and degeneracy.}
The three-dimensional (3D) unpolarized uniform electron gas (UEG) is parametrized by the Wigner--Seitz radius
$\rs=(3/4\pi n)^{1/3}$ in Bohr, with density
$n=3/(4\pi\rs^{3})$. The Fermi wavevector is
$\kF=(9\pi/4)^{1/3}/\rs$, the Fermi temperature
$\TF=\kF^{2}$ (Rydberg), and the reduced temperature
$\thetared=T/\TF$.

\paragraph*{Density of states.}
The $T=0$ density of states at the Fermi level is
$\Nf=\kF/(2\pi^{2})$. We use $\Nf$ throughout as the dimensionless
rescaling factor of the spin exchange-correlation (XC) kernel; the published variational diagrammatic Monte Carlo (VDMC) data
files store $\Kxc(q,0;\thetared)\cdot\Nf$ with $\Nf$ evaluated at $T=0$.

\paragraph*{Magnetization operator.}
We adopt $M=(n_{\uparrow}-n_{\downarrow})/2$ throughout, so that the
non-interacting static spin susceptibility at $q=0$ obeys
$\chinaught(q\!=\!0,0;T\!=\!0)=\Nf$.

\paragraph*{Spin XC kernel.}
The spin-antisymmetric (``$-$'') static XC kernel is defined by
\begin{equation}
    \Kxc(q,0;\thetared)\equiv\chis^{-1}(q,0;\thetared)-\chinaught^{-1}(q,0;\thetared),
    \label{eq:Kxc-def-sm}
\end{equation}
so that the static spin susceptibility enhancement reads
\begin{equation}
    \frac{\chis(0,0;\thetared)}{\chinaught(0,0;\thetared)}
    =\frac{1}{1+\Kxc(0,0;\thetared)\,\chinaught(0,0;\thetared)},
\end{equation}
with the finite-$T$ Lindhard function $\chinaught(0,0;\thetared)$ in the
denominator. The main-text Fig.~2 plots the dimensionless kernel
$-\Kxc(0,0;\thetared)\,\Nf$ directly, separating the kernel itself from
the additional finite-$T$ Lindhard factor. Stoner-enhanced
susceptibility ($\chis>\chinaught$) corresponds to $\Kxc<0$; our
data files store $\Kxc\cdot\Nf$ which is therefore negative for
metallic $\rs$.

\paragraph*{Local-field factor.}
The kernel and the spin-channel local-field factor (LFC) $G^{-}(q)$
are related via
\begin{equation}
    \Kxc(q,0;\thetared)=-\frac{8\pi}{q^{2}}\,G^{-}(q,0;\thetared).
\end{equation}
The unpolarized electron gas has $G^{-}(q\!\to\!0,T\!=\!0)>0$, so
$\Kxc(0,0;T\!=\!0)<0$ as required by Stoner enhancement.

\paragraph*{Uniform-limit identity.}
Under the conventions above, the small-$\zeta$ expansion of the XC
free energy per electron $\fxc(\rs,\thetared,\zeta)$ in Rydberg reads
\begin{equation}
    \fxc(\rs,\thetared,\zeta)=\fxc(\rs,\thetared,0)+
    \tfrac{1}{2}\,\axc(\rs,\thetared)\,\zeta^{2}+O(\zeta^{4}),
    \qquad
    \axc(\rs,\thetared)\equiv\frac{\partial^{2}\fxc}{\partial\zeta^{2}}\bigg|_{\zeta=0},
    \label{eq:axc-def-sm}
\end{equation}
and likewise for the kinetic-entropy contribution $f_{0}(\rs,\thetared,\zeta)$
of the non-interacting Fermi gas, with curvature
$\alpha_{0}(\rs,\thetared)\equiv\partial^{2}f_{0}/\partial\zeta^{2}|_{\zeta=0}$.
Define a uniform external field $h$ which couples to the
spin-density imbalance through
\begin{equation}
    \delta\hat H = -h\!\int\!d\mathbf{r}\,\bigl[n_{\uparrow}(\mathbf{r})-n_{\downarrow}(\mathbf{r})\bigr]
    = -2h\!\int\!d\mathbf{r}\,M(\mathbf{r}),
    \label{eq:Zeeman-sm}
\end{equation}
so that $h$ is conjugate to the symmetrised difference
$n_{\uparrow}-n_{\downarrow}=n\zeta$, not to our magnetization
operator $M=(n_{\uparrow}-n_{\downarrow})/2=n\zeta/2$. With this
choice the total free energy density is
\begin{equation}
    \omega(\zeta;\rs,T,h)
    = n\bigl[f_{0}(\rs,\thetared,\zeta)+\fxc(\rs,\thetared,\zeta)\bigr]-h\,n\,\zeta,
\end{equation}
and minimization in $\zeta$ at fixed $n$ gives, to leading order,
\begin{equation}
    \bigl[\alpha_{0}(\rs,\thetared)+\axc(\rs,\thetared)\bigr]\,\zeta=h
    \quad\Longrightarrow\quad
    M=\frac{n\zeta}{2}=\frac{n\,h}{2[\alpha_{0}+\axc]}.
\end{equation}
The static spin susceptibility, defined as the response of $M$ to
$h$, is therefore
\begin{equation}
    \chis(0,0;\thetared)=\frac{\partial M}{\partial h}\bigg|_{h=0}
    =\frac{n}{2[\alpha_{0}(\rs,\thetared)+\axc(\rs,\thetared)]},
    \qquad
    \chinaught(0,0;\thetared)=\frac{n}{2\alpha_{0}(\rs,\thetared)}.
    \label{eq:chi-of-alpha-sm}
\end{equation}
Inverting Eq.~(\ref{eq:chi-of-alpha-sm}) and using the
definition~(\ref{eq:Kxc-def-sm}) yields the uniform-limit identity
\begin{equation}
    \Kxc(0,0;\thetared)=\chis^{-1}-\chinaught^{-1}
    =\frac{2[\alpha_{0}+\axc]-2\alpha_{0}}{n}
    =\frac{2\,\axc(\rs,\thetared)}{n}.
    \label{eq:uniform-limit-sm}
\end{equation}

\paragraph*{PIMC comparison.}
For the path-integral Monte Carlo (PIMC) comparison in Fig.~1(b) of
the main text, we use the $\rs=2$, $\thetared=1$ data of
Dornheim et al.~\cite{Dornheim2022spin,Dornheim2022rodare}. These
data are reported as spin-resolved static local-field factors
$G_{\uparrow\uparrow}(q,0;\thetared)$ and
$G_{\uparrow\downarrow}(q,0;\thetared)$. We form
$G^{-}(q,0;\thetared)\equiv
    [G_{\uparrow\uparrow}-G_{\uparrow\downarrow}]/2$ under the convention
above and use $\Kxc=-(8\pi/q^2)G^{-}$ to obtain the gray triangles in
that panel. The finite-size analysis reported in
Ref.~\cite{Dornheim2022spin} indicates small size effects for the
analyzed spin-resolved response quantities, so the published static
spin-LFC values are used without an additional finite-size correction.
The comparison combines data sets with different methods, momentum
grids, and finite-size treatments, and is therefore used only as a
qualitative external consistency check.

%% =================================================================
\section{\texorpdfstring{Analytic XC spin stiffness from GDB and corrKSDT}
  {Analytic XC spin stiffness from GDB and corrKSDT}}\label{sec:alpha}
%% =================================================================

Both Groth--Dornheim et al. (GDB)~\cite{Groth2017} and the Karasiev--Sjostrom--Dufty--Trickey (KSDT) family use the
Perrot--Dharma--Wardana (PDW) spin-interpolation ansatz
\begin{equation}
    \fxc(\rs,\thetared,\zeta)=\fxc^{\zeta=0}(\rs,\thetared)+
    \bigl[\fxc^{\zeta=1}(\rs,2^{-2/3}\thetared)-\fxc^{\zeta=0}(\rs,\thetared)\bigr]
    \,\varphi(\rs,\thetared,\zeta),
\end{equation}
with
\begin{equation}
    \varphi(\rs,\thetared,\zeta)=
    \frac{(1+\zeta)^{\pexp}+(1-\zeta)^{\pexp}-2}{2^{\pexp}-2},
    \qquad \pexp=\pexp(\rs,\thetared).
\end{equation}
The exponent $\pexp(\rs,\thetared)$ is the spin-polarization interpolation
exponent (\emph{not} the spin stiffness $\axc$). GDB and the KSDT
family parametrize it with the PDW form
$\pexp=2-g(\rs)\exp[-\thetared\lambda(\rs,\thetared)]$, but with different
coefficients (see the tables of Refs.~\cite{Groth2017,KSDT2014}).
For corrKSDT we use the corrected finite-temperature UEG
parametrization of Ref.~\cite{Karasiev2018}. Since only the
$\varphi(\zeta)$ factor carries $\zeta$ dependence, the second
derivative at $\zeta=0$ is analytic,
\begin{equation}
    \axc(\rs,\thetared)=
    \bigl[\fxc^{\zeta=1}(\rs,2^{-2/3}\thetared)-\fxc^{\zeta=0}(\rs,\thetared)\bigr]
    \cdot\varphi''(0;\pexp),
    \qquad
    \varphi''(0;\pexp)=\frac{2\pexp(\pexp-1)}{2^{\pexp}-2}.
    \label{eq:axc-analytic}
\end{equation}
We have verified Eq.~(\ref{eq:axc-analytic}) against a symmetric
finite difference,
$\axc\approx 2[\fxc(\rs,\thetared,\varepsilon)-\fxc(\rs,\thetared,0)]/\varepsilon^{2}$
with $\varepsilon=10^{-2}$ (using that $\fxc$ is even in $\zeta$);
relative agreement is better than $10^{-5}$ across
$\rs\in\{1,2,3,4\}$ and $\thetared\in\{0.04,\dots,8\}$ for both fits.
All thermodynamic-closure curves shown in
Fig.~2 of the main text are produced from
Eq.~(\ref{eq:axc-analytic}).

\paragraph*{corrKSDT implementation check.}
The corrKSDT curves in Fig.~2 of the main text are obtained by
evaluating the published corrKSDT parametrization and applying
Eq.~(\ref{eq:axc-analytic}). Our implementation reproduces the
published corrKSDT--GDB scalar free-energy comparison on the
metallic-density and temperature window studied here~\cite{Karasiev2019}.

\paragraph*{Where the spin curvature is constrained in GDB and corrKSDT.}
The response benchmark in Fig.~2 of the main text tests a quantity
that is not directly fitted in either LSDA parametrization. In
corrKSDT, the finite-$T$ spin dependence follows the KSDT PDW
interpolation structure; finite-$T$ partial-polarization data do not
directly constrain the $\zeta=0$ curvature. GDB includes finite-$T$
partial-polarization QMC information~\cite{Groth2017}, but still
represents the spin dependence with a single-parameter PDW
interpolation. Consequently, the values of $\fxc$ at finite
polarization can be fitted while the local curvature
$\axc=\partial_{\zeta}^{2}\fxc|_{\zeta=0}$ remains an
ansatz-dependent consequence of the interpolation. The VDMC
$\Kxc(0,0;\thetared)$ data therefore provide an independent
second-derivative response constraint on this curvature.

%% =================================================================
\section{VDMC convergence and uncertainty estimate}\label{sec:convergence}
%% =================================================================

The reported $\Kxc(q;\thetared)\,\Nf$ error bars are evaluated at the
principle-of-minimal-sensitivity (PMS) selected Yukawa scale
$\lambda_{\rm opt}(q)$ and combine the VDMC statistical uncertainty
with the last-order truncation estimate $|K_{xc}^{-,(5)}-K_{xc}^{-,(4)}|\,\Nf$.
The $\lambda$ dependence is used as a PMS stability diagnostic.
Figure~\ref{fig:sm-convergence} documents
both the order convergence and the $\lambda$ stability at $\rs=4$
--- the strongest-coupling density in the analysis and therefore the
worst-case convergence demonstration --- across low-temperature
($\thetared=0.125$), warm ($\thetared=1$), and high-temperature
($\thetared=4$) cases, at $q=0$ (top row; the quantity entering
Fig.~2 of the main text) and at $q=2\kF$ (bottom row; the
Fermi-surface feature visible in Fig.~1). The same pattern holds at
$\rs=1,2,3$ with the optimal Yukawa scale $\lambda_{\rm opt}$
shifting to correspondingly larger values consistent with the
density-dependence of the Coulomb coupling.

At $\thetared=0.125$ and $\thetared=1$, the order-by-order partial
sums through $N=5$ converge to a stable plateau at
$\lambda\in[0.25,0.50]$ for $\rs=4$, at both $q=0$ and $q=2\kF$.
Across the resolved PMS plateau, the values vary smoothly and remain
small on the scale of the temperature evolution and of the
high-temperature VDMC--GDB residuals discussed in the main text,
supporting the use of the PMS-selected $\lambda_{\rm opt}$ values.

At high temperatures (panels c, f at $\thetared=4$; analogous
behavior at $\thetared=8$), the diagrammatic series converges
substantially faster: the order-$N=5$ truncation contribution
$|a_5|\,\Nf$, where $|a_5|$ is the difference of the $N=4$ and
$N=5$ partial sums on $\Kxc$, is small compared with the
high-temperature residuals discussed in Fig.~2 of the main text,
reflecting the expected suppression of interaction effects as the
system approaches the classical limit. In this regime the rapid order
convergence makes the PMS-selected $\lambda_{\rm opt}$ estimate stable at
the level relevant for the main-text comparisons.

\paragraph*{Uncertainty quoted throughout this work.}
The error bar reported on $\Kxc(q;\thetared)\,\Nf$ at every
$(\rs,\thetared,q)$ throughout the main text and this SM is the
quadrature sum of the VDMC statistical uncertainty at
$\lambda_{\rm opt}(q)$ and the magnitude of the order-$N=5$
truncation contribution, i.e.\ the difference of the partial sums at
$N=4$ and $N=5$ multiplied by $\Nf$. The $\lambda$ scans shown here
verify that the reported values lie on stable PMS plateaus where
resolved, while the high-temperature cases are already visually
converged on the scale relevant for the main-text comparisons.

\begin{figure}[h]
    \centering
    \includegraphics[width=0.99\textwidth]{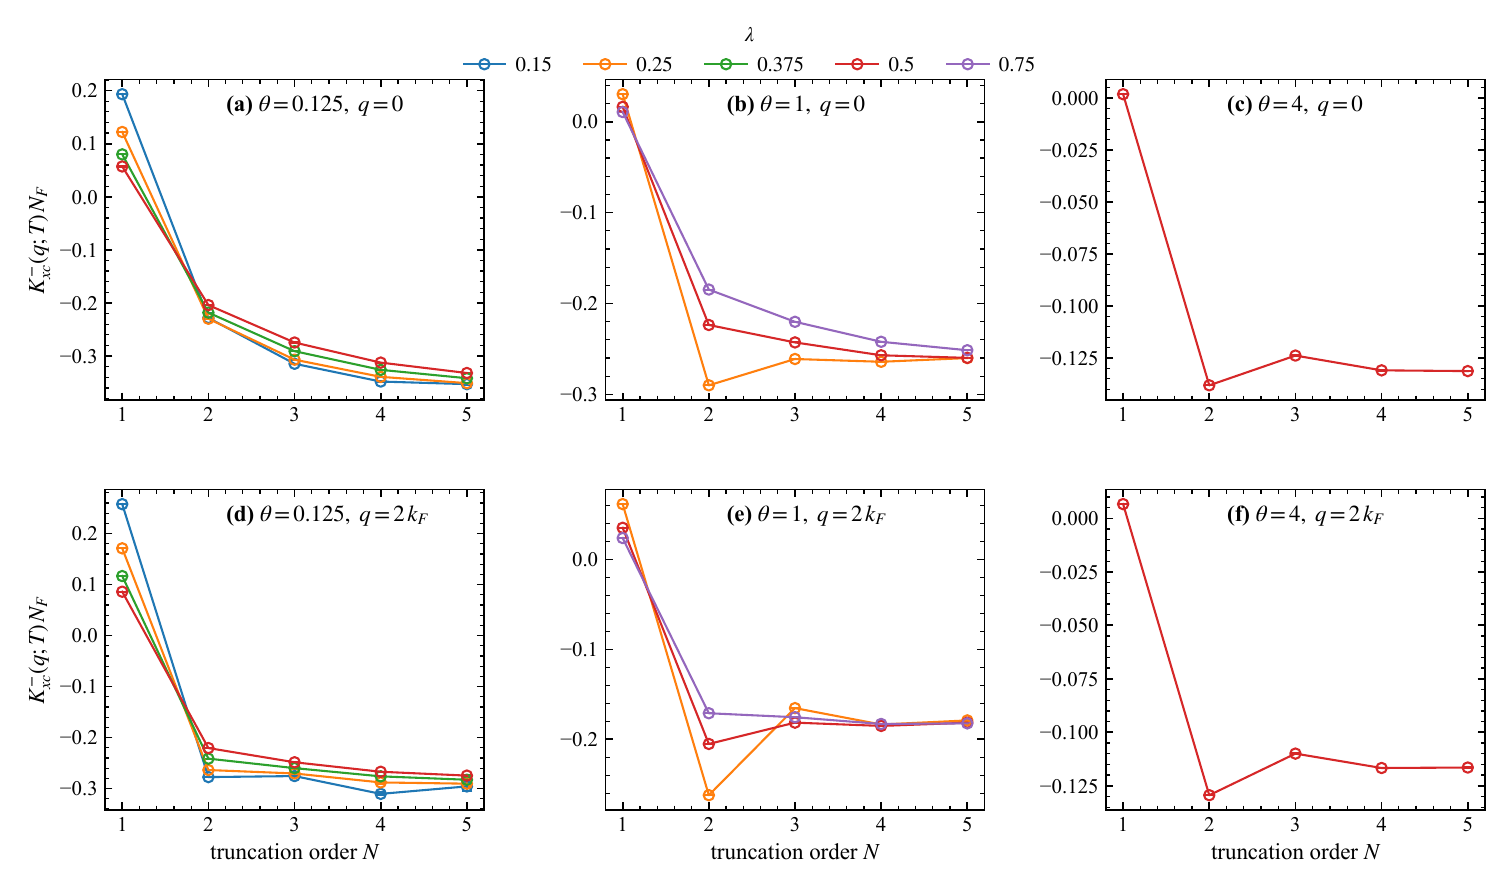}
    \caption{\label{fig:sm-convergence}%
        Variational diagrammatic Monte Carlo (VDMC) truncation-order
        convergence at $\rs=4$, the
        strongest-coupling density in the analysis: top row at
        $q=0$, bottom row at $q=2\kF$; columns at $\thetared=0.125$
        (a, d), $\thetared=1$ (b, e), and $\thetared=4$ (c, f).
        Each curve plots $\Kxc(q;\thetared)\,\Nf$ as a function of
        truncation order $N$ at fixed $\lambda$ in units of $\kF$.
        Computation: $\Kxc=1/\chi^{(N)}_s-1/\chi_0$ with
        $\chi^{(N)}_s$ the order-$N$ partial sum of the spin
        susceptibility and $\chi_0$ the non-interacting bubble. The
        PMS plateau is visible at
        $\lambda\in[0.25,0.50]$ at both
        $\thetared=0.125$ and $\thetared=1$; at $\thetared=4$ only
        $\lambda_{\rm opt}$ is shown because the order-by-order
        series is already visually converged on the scale of the
        plotted data (see text).
        Statistical error bars are smaller than the markers.}
\end{figure}

%% =================================================================
\section{\texorpdfstring{VDMC-constrained PDW spin-interpolation exponent
      $\pexp_{\star}(\rs,\thetared)$}
  {VDMC-constrained PDW spin-interpolation exponent p-star}}\label{sec:pstar}
%% =================================================================

Inverting Eqs.~(\ref{eq:uniform-limit-sm}) and~(\ref{eq:axc-analytic})
for $\pexp$ at every $(\rs,\thetared)$ on the VDMC grid defines a
response-constrained diagnostic exponent
$\pexp_{\star}(\rs,\thetared)$ \emph{within the PDW
    interpolation form}. This inversion is not an independent
parametrization of the spin-polarized free energy: it fixes the
scalar free-energy difference $\fxc^{\zeta=1}-\fxc^{\zeta=0}$ as an
external input and asks which PDW exponent would reproduce the VDMC
$q=0$ spin curvature. We therefore report two inversions, one with
the GDB scalar endpoints and one with the corrKSDT scalar endpoints, and
combine the two into a single \emph{systematic band} that brackets
the VDMC statistical 1-$\sigma$ envelopes around both. The map
$\pexp\mapsto\varphi''(0;\pexp)=2\pexp(\pexp-1)/(2^{\pexp}-2)$ is
strictly monotonic on the physical branch $\pexp\in(1,2]$ in which
both GDB and corrKSDT lie; entries for which the inverted
$\varphi''(0;\pexp)$ falls outside this branch are clipped to the
boundary and flagged with an asterisk in
Table~\ref{tab:pstar-rep}. Clipped values do not carry a meaningful
statistical uncertainty and should be read only as one-sided bounds
for this diagnostic.

Figure~\ref{fig:pstar} compares the resulting $\pexp_{\star}$ with
the GDB and corrKSDT exponents and with the pure-exchange limit
$\pexp=4/3$, one panel per density across $\rs=1$--$4$.
Representative numerical values are listed in
Table~\ref{tab:pstar-rep}; the full inversion grid is included in
the data deposit. The direct VDMC--GDB residual on
$\Kxc(0;\thetared)\,\Nf$ underlying this PDW-dependent inversion is
displayed in the bottom panel of Fig.~2 of the main text.

\begin{figure}[h]
    \centering
    \includegraphics[width=0.82\textwidth]{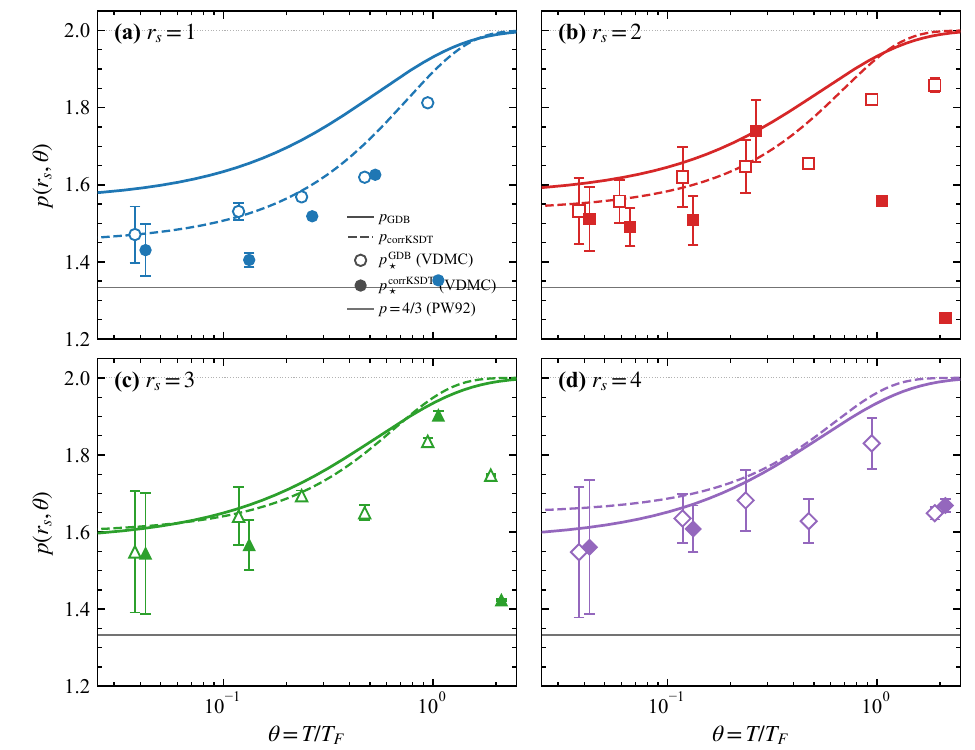}
    \caption{\label{fig:pstar}%
        VDMC-constrained, ansatz-dependent PDW spin-interpolation exponent
        $\pexp_{\star}(\rs,\thetared)$ versus reduced temperature
        $\thetared=T/\TF$, one panel per density (a)~$\rs=1$,
        (b)~$\rs=2$, (c)~$\rs=3$, (d)~$\rs=4$. Solid (dashed) colored
        curves are the exponents from the Groth--Dornheim et al. (GDB)
        and corrKSDT parametrizations~\cite{KSDT2014,Karasiev2018}. Open
        (filled) markers are the VDMC inversions using the GDB
        (corrKSDT) scalar endpoints, slightly offset on the log-$\theta$
        axis so the two inversions are visually separated; error bars
        are the propagated VDMC 1-$\sigma$ statistical envelope only,
        so the open--filled spread isolates the GDB$\leftrightarrow$corrKSDT
        scalar-fit systematic. Horizontal gray line: pure-exchange limit
        $\pexp=4/3$ from PW92~\cite{PerdewWang1992}; dotted line:
        PDW saturation $\pexp=2$. High-temperature
        points with $\thetared>2$ are omitted because the inversion
        can saturate against the physical-branch endpoints and then
        ceases to convey quantitative information; the full numerical grid
        is included in the data deposit.}
\end{figure}

\begin{table}[h]
    \centering
    \caption{\label{tab:pstar-rep}%
        Representative VDMC-constrained PDW spin-interpolation
        exponents $\pexp_{\star}(\rs,\thetared)$ from
        Eqs.~(\ref{eq:uniform-limit-sm})--(\ref{eq:axc-analytic}).
        The GDB and corrKSDT columns use the corresponding scalar
        endpoints $\fxc^{\zeta=0,1}$ separately. The band brackets both
        endpoint choices and their propagated 1-$\sigma$ VDMC statistical
        envelopes. Asterisks mark physical-branch endpoint bounds rather
        than fitted exponents.}
    \begin{tabular}{c c c c c c c c}
        \toprule
        $\rs$                     & $\thetared$                    & $\Kxc\,\Nf$ (VDMC)  &
        $\pexp_{\rm GDB}$         & $\pexp_{\rm corrKSDT}$         &
        $\pexp_{\star}^{\rm GDB}$ & $\pexp_{\star}^{\rm corrKSDT}$ &
        band $[p_{\rm lo}, p_{\rm hi}]$                                                                                                                           \\
        \midrule
        1                         & 0.040                          & $-0.1319\pm 0.0030$ & 1.591 & 1.472 & $1.471\pm 0.073$ & $1.489\pm 0.075$ & $[1.398, 1.564]$ \\
        1                         & 1.000                          & $-0.1192\pm 0.0001$ & 1.931 & 1.893 & $1.813\pm 0.007$ & $1.626\pm 0.005$ & $[1.621, 1.819]$ \\
        1                         & 4.000                          & $-0.0552\pm 0.0002$ & 2.000 & 2.000 & $1.937\pm 0.023$ & $1.723\pm 0.015$ & $[1.709, 1.960]$ \\
        \midrule
        2                         & 0.040                          & $-0.2271\pm 0.0056$ & 1.604 & 1.553 & $1.532\pm 0.086$ & $1.567\pm 0.092$ & $[1.445, 1.659]$ \\
        2                         & 1.000                          & $-0.1860\pm 0.0002$ & 1.933 & 1.928 & $1.821\pm 0.006$ & $2.000^{\ast}$   & $[1.815, 2.000]$ \\
        2                         & 4.000                          & $-0.0900\pm 0.0006$ & 2.000 & 2.000 & $1.746\pm 0.033$ & $1.867\pm 0.042$ & $[1.713, 1.909]$ \\
        \midrule
        3                         & 0.040                          & $-0.2993\pm 0.0128$ & 1.608 & 1.614 & $1.549\pm 0.157$ & $1.593\pm 0.170$ & $[1.391, 1.764]$ \\
        3                         & 1.000                          & $-0.2302\pm 0.0004$ & 1.934 & 1.948 & $1.835\pm 0.009$ & $2.000^{\ast}$   & $[1.826, 2.000]$ \\
        3                         & 4.000                          & $-0.1169\pm 0.0021$ & 2.000 & 2.000 & $1.758\pm 0.093$ & $2.000^{\ast}$   & $[1.665, 2.000]$ \\
        \midrule
        4                         & 0.040                          & $-0.3560\pm 0.0163$ & 1.611 & 1.663 & $1.548\pm 0.169$ & $1.599\pm 0.186$ & $[1.378, 1.785]$ \\
        4                         & 1.000                          & $-0.2599\pm 0.0028$ & 1.935 & 1.961 & $1.830\pm 0.066$ & $2.000^{\ast}$   & $[1.764, 2.000]$ \\
        4                         & 4.000                          & $-0.1313\pm 0.0004$ & 2.000 & 2.000 & $1.583\pm 0.011$ & $1.909\pm 0.020$ & $[1.573, 1.929]$ \\
        \bottomrule
    \end{tabular}
\end{table}

At low temperature the inferred bands overlap the exponents from GDB
and corrKSDT within the propagated VDMC uncertainty, consistent with
the low-temperature agreement in Fig.~2 of the main text. In the
warm-dense regime the
GDB-endpoint inversion lies below the GDB exponent as the
latter approaches its saturation value $\pexp=2$, indicating within
the PDW form a faster-than-VDMC thermal evolution of the fitted spin
interpolation. The separation between the GDB- and
corrKSDT-endpoint inversions in Table~\ref{tab:pstar-rep} shows the
associated scalar-endpoint sensitivity; it is included in the
reported bands and does not alter the qualitative trend. A
self-consistent finite-$T$ spin parametrization would need to combine
the present $\Kxc(0;\thetared)$ response constraints with the
partial-polarization QMC data underlying the existing LSDA fits.

%% =================================================================
\section{Classical high-temperature limits}\label{sec:highT-asymptote}
%% =================================================================

The contrast between the spin and charge channels in
Fig.~3 of the main text---the spin kernel becoming nearly
$q$-independent on the Fermi-momentum scale at $\thetared\gtrsim 4$
while the $\rs=1$ charge-kernel comparison retains a pronounced
$q$-shape---follows from the different role of the Coulomb
interaction in the two channels: it is spin-blind, but long-ranged in
charge. We summarize the corresponding high-$T$ classical limits
here~\cite{GiulianiVignale2005,Ichimaru1987,
    PerrotDharmawardana2000}.

\paragraph*{Spin sector: Curie limit.}
At $\thetared\to\infty$ the system becomes classical and the
electrons obey Maxwell--Boltzmann statistics. Under the
$M=(n_\uparrow-n_\downarrow)/2$ convention of Sec.~\ref{sec:convention}
and the Zeeman coupling $\delta\hat H=-h\int d\mathbf{r}\,
    (n_\uparrow-n_\downarrow)$ of Eq.~(\ref{eq:Zeeman-sm}), the
non-interacting susceptibility at $q=0$ obeys
$\chinaught(0,0;\thetared)=n/[2\alpha_0(\rs,\thetared)]$ from
Eq.~(\ref{eq:chi-of-alpha-sm}), with the classical limit
$\alpha_0(\rs,T\!\to\!\infty)=T+O(1/T)$ from the leading
spin-mixing entropy of an ideal $s=\tfrac12$ Maxwell--Boltzmann
gas. Hence
\begin{equation}
    \chinaught(q,0;T\!\to\!\infty) = \frac{n}{2T} + \mathcal{O}(1/T^2),
\end{equation}
$q$ independent on the Fermi-momentum scale to leading order in
$1/T$, since the thermal de Broglie wavelength
$\lambda_T=(2\pi/(mT))^{1/2}\ll 1/\kF$. Because the Hamiltonian
contains no spin-dependent coupling, Coulomb interactions cannot
change this leading-order Curie form, so the interacting
susceptibility obeys the same identity at leading order,
\begin{equation}
    \chis(q,0;T\!\to\!\infty) = \chinaught(q,0;T\!\to\!\infty)
    + \mathcal{O}(1/T^2),
\end{equation}
with the subleading correction generated by quantum exchange and
correlation effects, the only mechanisms coupling spin to dynamics in
this limit. The $q$-structure of the leading nonvanishing $\Kxc(q,0;\thetared)$
at high $T$ is set by the thermal de Broglie wavelength
$\lambda_T=(2\pi/(mT))^{1/2}$~\cite{Ichimaru1987,GiulianiVignale2005};
since $\lambda_T\kF\to 0$ for $\thetared\gg 1$, the leading
coefficient is flat on the Fermi-momentum scale up to corrections
of order $(\lambda_T\kF)^2=\mathcal{O}(1/\thetared)$. Both
$\Kxc(q;\thetared)$ and $\Kxc(0;\thetared)$ inherit this flatness, so the
normalized ratio approaches
\begin{equation}
    \lim_{\thetared\to\infty}\frac{\Kxc(q;\thetared)}{\Kxc(0;\thetared)} = 1
    \quad \text{for } q \lesssim 2\kF,
    \label{eq:curie-ratio}
\end{equation}
i.e.\ a horizontal line at unity (the \emph{Curie asymptote}),
with corrections suppressed by $\mathcal{O}(1/\thetared)$.
Figure~3(b) of the main text shows the VDMC ratio approaching this
line for $\thetared\gtrsim 4$ within $\sim 10\%$ across $q\le 2\kF$,
consistent with the predicted $\mathcal{O}(1/\thetared)$
suppression.

\paragraph*{Charge sector: Coulomb-imposed $q$-structure.}
The same classical limit applied to the charge response gives the
Debye--H\"uckel form~\cite{Ichimaru1987,TanakaIchimaru1986}
\begin{equation}
    \chi_n^{\rm cl}(q,0;T) = \frac{n}{T}\,\frac{q^2}{q^2+\kappa_D^2},
    \qquad \kappa_D^2 = 8\pi n/T,
\end{equation}
which retains an explicit $q$-shape set by the Debye wavevector
$\kappa_D$. Thus the charge response carries the long-range Coulomb
scale even in the classical regime. Beyond RPA, the charge local-field
correction $G^+(q;T)$ adds additional structure from short-range
correlations in the classical one-component plasma at finite
coupling~\cite{Ichimaru1987,TanakaIchimaru1986}. In the strict
high-$T$ RPA limit $\KxcPlus(q;T)\to 0$ identically, so the empirical
ratio $\KxcPlus(q;T)/\KxcPlus(0;T)$ shown in Fig.~3(a) of the main
text does not have a universal Curie-like asymptote analogous to
Eq.~(\ref{eq:curie-ratio}). The relevant point for the present
comparison is therefore channel asymmetry: the charge response
inherits Coulomb $q$ scales, whereas no corresponding bare
spin-channel scale exists because the Coulomb interaction does not
couple to the spin-antisymmetric channel.

%% =================================================================
\section{Density dependence of high-temperature spin-kernel locality}\label{sec:locality-rs}
%% =================================================================

Figure~\ref{fig:sm-locality-rs} extends the spin panel of Fig.~3 of
the main text from $\rs=1$ to $\rs=2,3,4$, demonstrating that the
temperature-driven crossover to a near-flat normalized spin kernel
for $\thetared\gtrsim 4$ is robust across the metallic-density
window. At each density the $\thetared=0.25$ curve retains a residual
$2\kF$-like hump above unity, whose amplitude decreases
monotonically with $\rs$ and is absent by $\rs=4$. The strongest
$q$-dependence at every density occurs at
$\thetared\simeq 0.5$--$1$. By $\thetared\gtrsim 4$ the normalized
spin kernel stays within $\sim 10\%$ of unity over $q\le 2\kF$ at all
four densities, tightening to within $\sim 5\%$ by $\thetared=8$,
and the residual $q$-profile is essentially $\rs$-independent within
the probed window.

\begin{figure}
    \centering
    \includegraphics[width=0.82\textwidth]{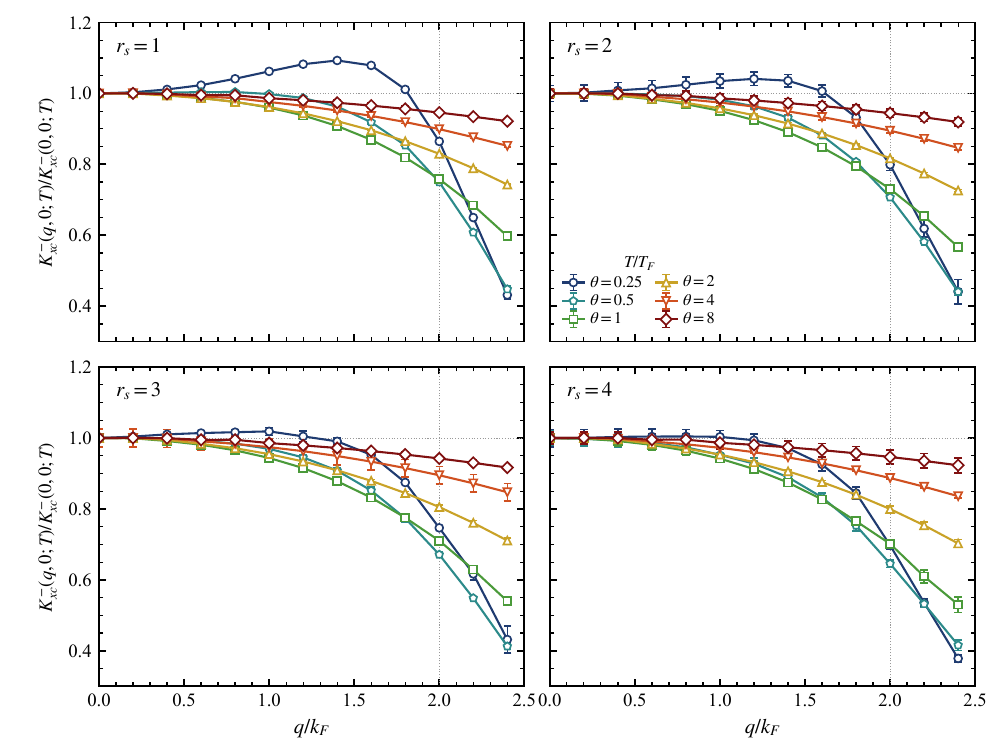}
    \caption{\label{fig:sm-locality-rs}%
        Normalized static spin exchange-correlation (XC) kernel
        $\Kxc(q,0;\thetared)/\Kxc(0,0;\thetared)$ vs $q/\kF$ for $\rs\in\{1,2,3,4\}$
        and a common temperature grid
        $\thetared\in\{0.25,0.5,1,2,4,8\}$. The temperature-driven
        flattening for $\thetared\gtrsim 4$ is present at every
        density, supporting the $\rs$-independence of the emergent
        thermal locality crossover described in the main text.}
\end{figure}

\bibliographystyle{apsrev4-2}
\bibliography{references}

\end{document}
